# Supplementary material for: Verifying Verified Code
Source: arXiv:2107.00723 source file (2021-07-01)
Supplement: Supplementary file 10 [file fig-result-per-category.tex]

\begin{figure}[t]
  \centering
\begin{subfigure}{.5\linewidth}
  \includegraphics[scale=0.38]{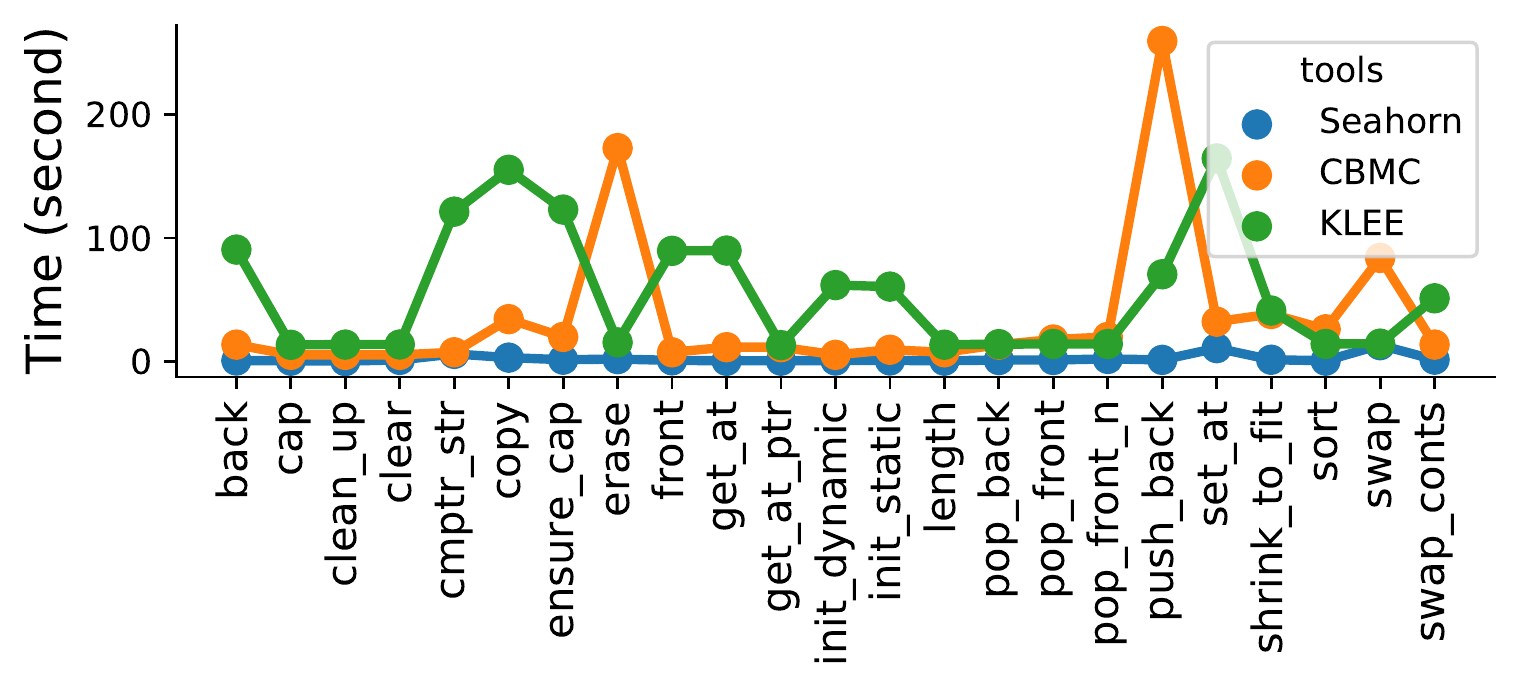}
  \caption{\code{aws_array_list}}
  \label{fig:comp_arylst}
\end{subfigure}%
\begin{subfigure}{.5\linewidth}
  \includegraphics[scale=0.35]{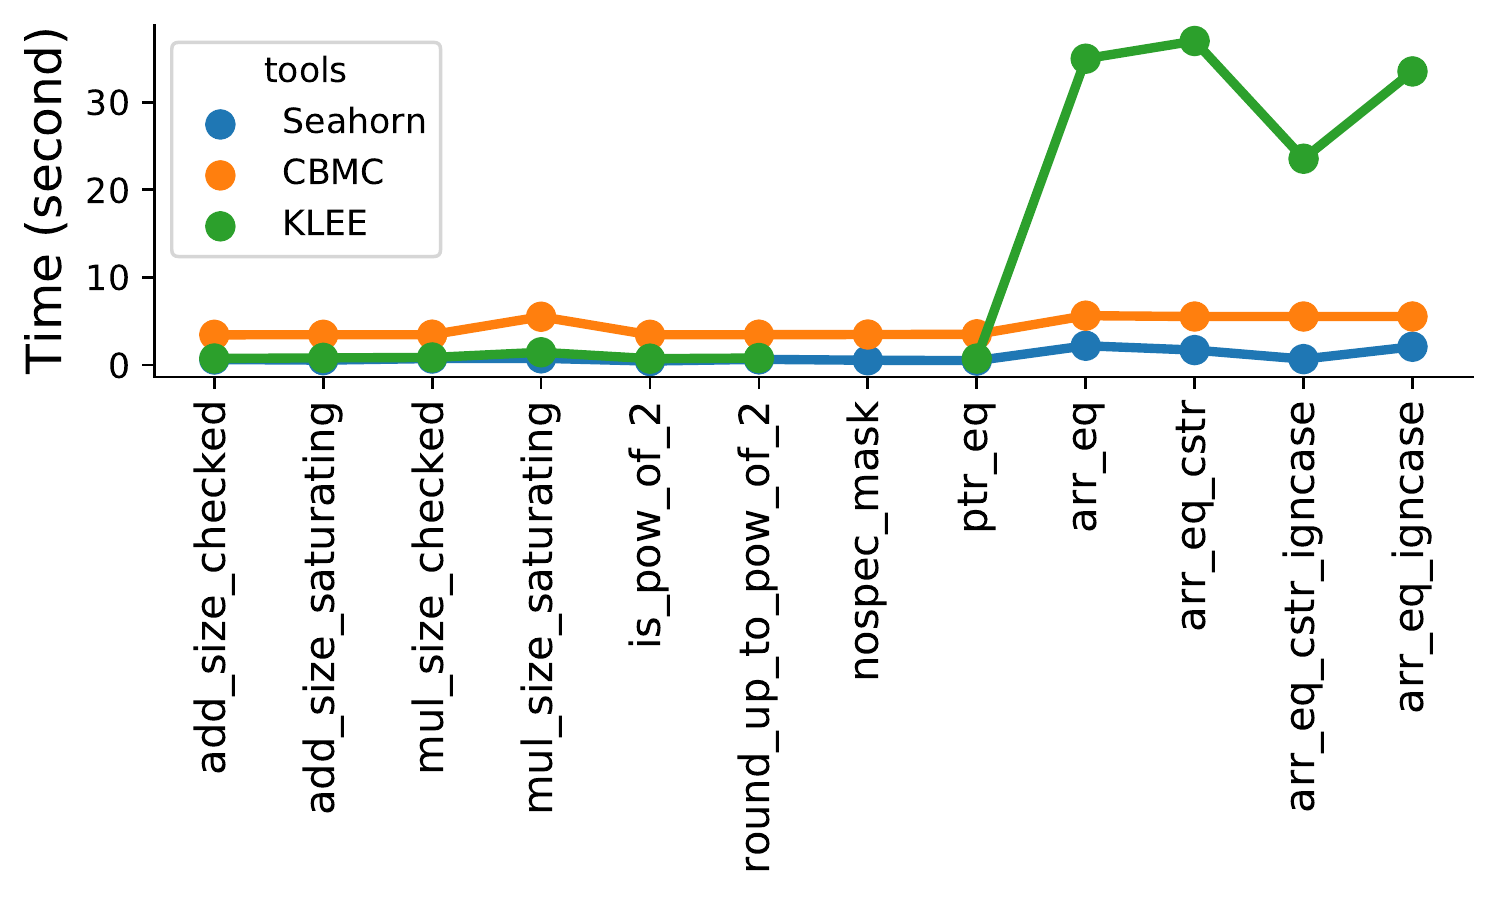}
  \caption{Others}
  \label{fig:comp_others}
\end{subfigure}%
\hfill
\begin{subfigure}{.5\linewidth}
  \includegraphics[scale=0.38]{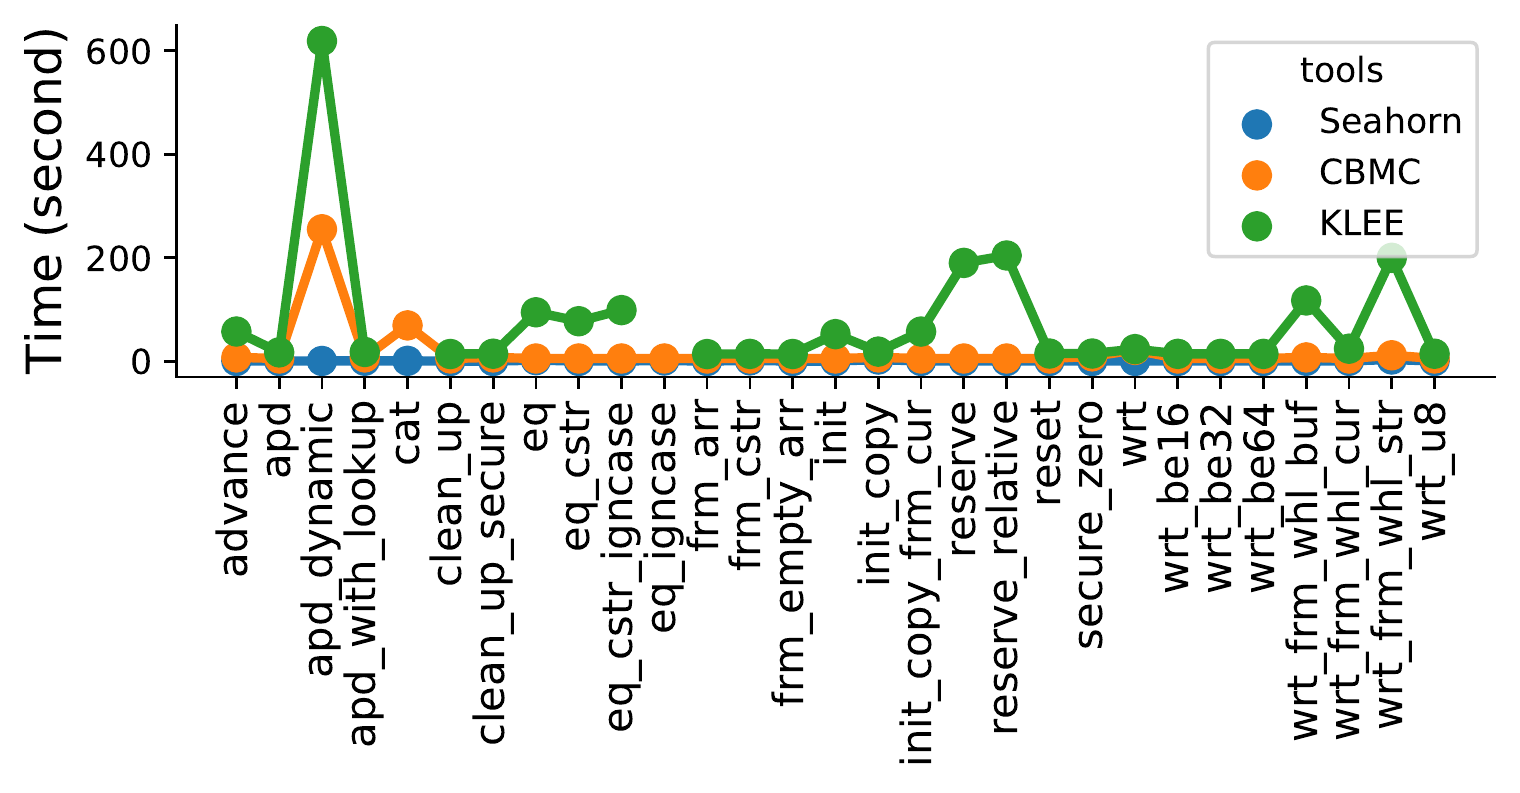}
  \caption{\code{aws_byte_buffer}}
  \label{fig:comp_bytebuf}
\end{subfigure}%
\begin{subfigure}{.5\linewidth}
  \includegraphics[scale=0.35]{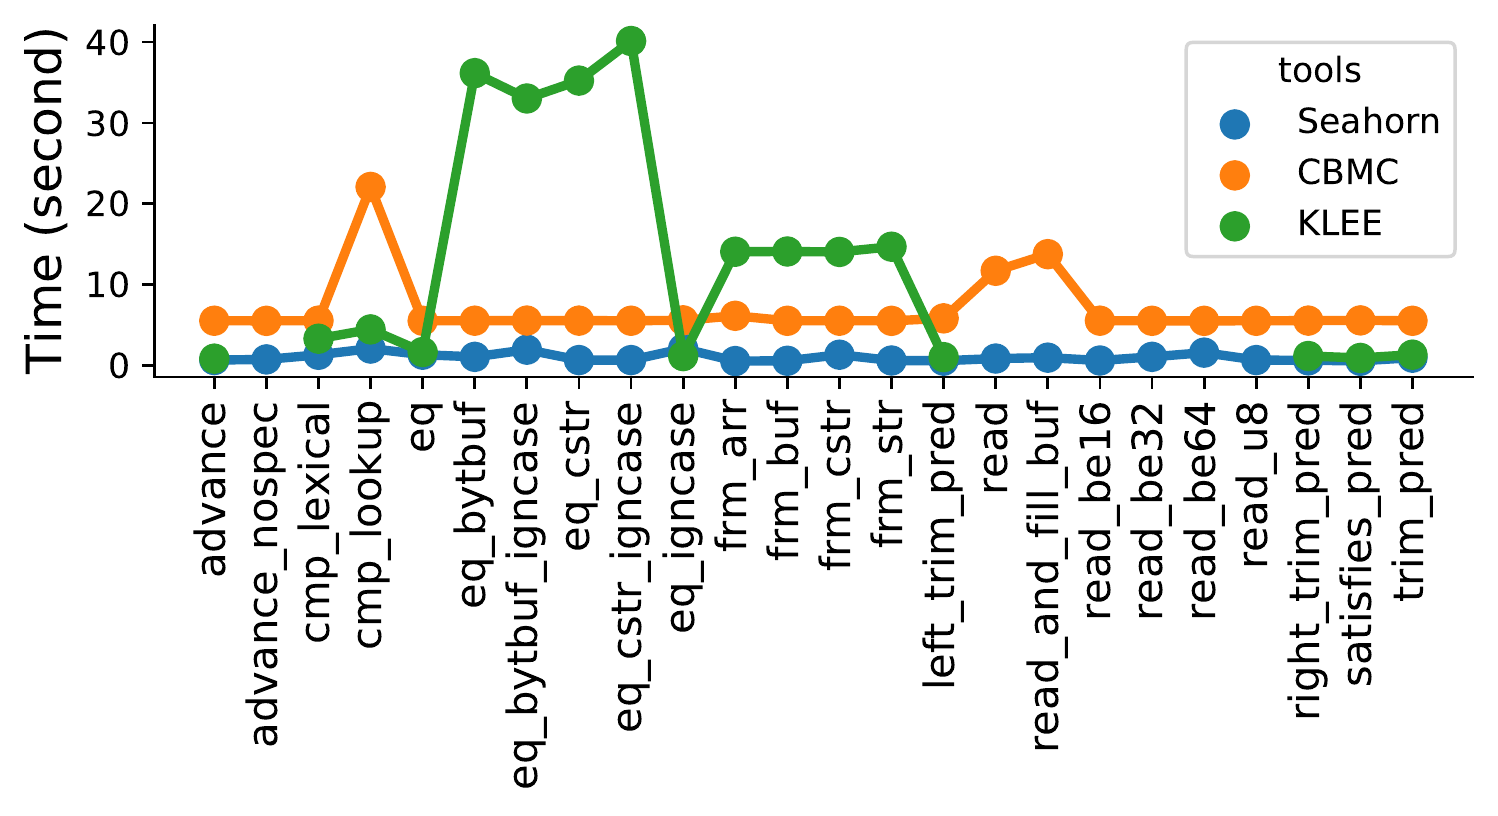}
  \caption{\code{aws_byte_cursor}}
  \label{fig:comp_bytecursor}
\end{subfigure}%
\hfill
\begin{subfigure}{.5\linewidth}
  \includegraphics[scale=0.38]{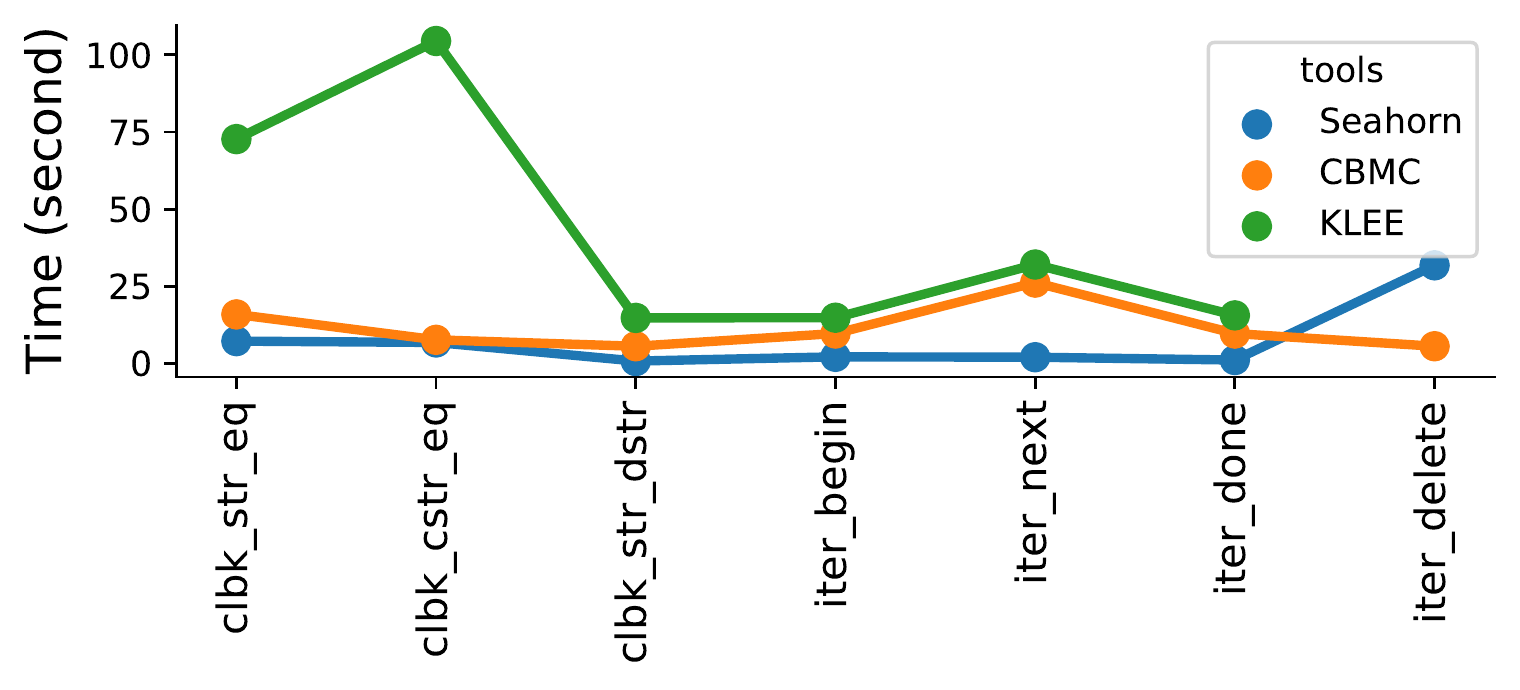}
  \caption{Hash}
  \label{fig:comp_hash}
\end{subfigure}%
\begin{subfigure}{.5\linewidth}
  \includegraphics[scale=0.35]{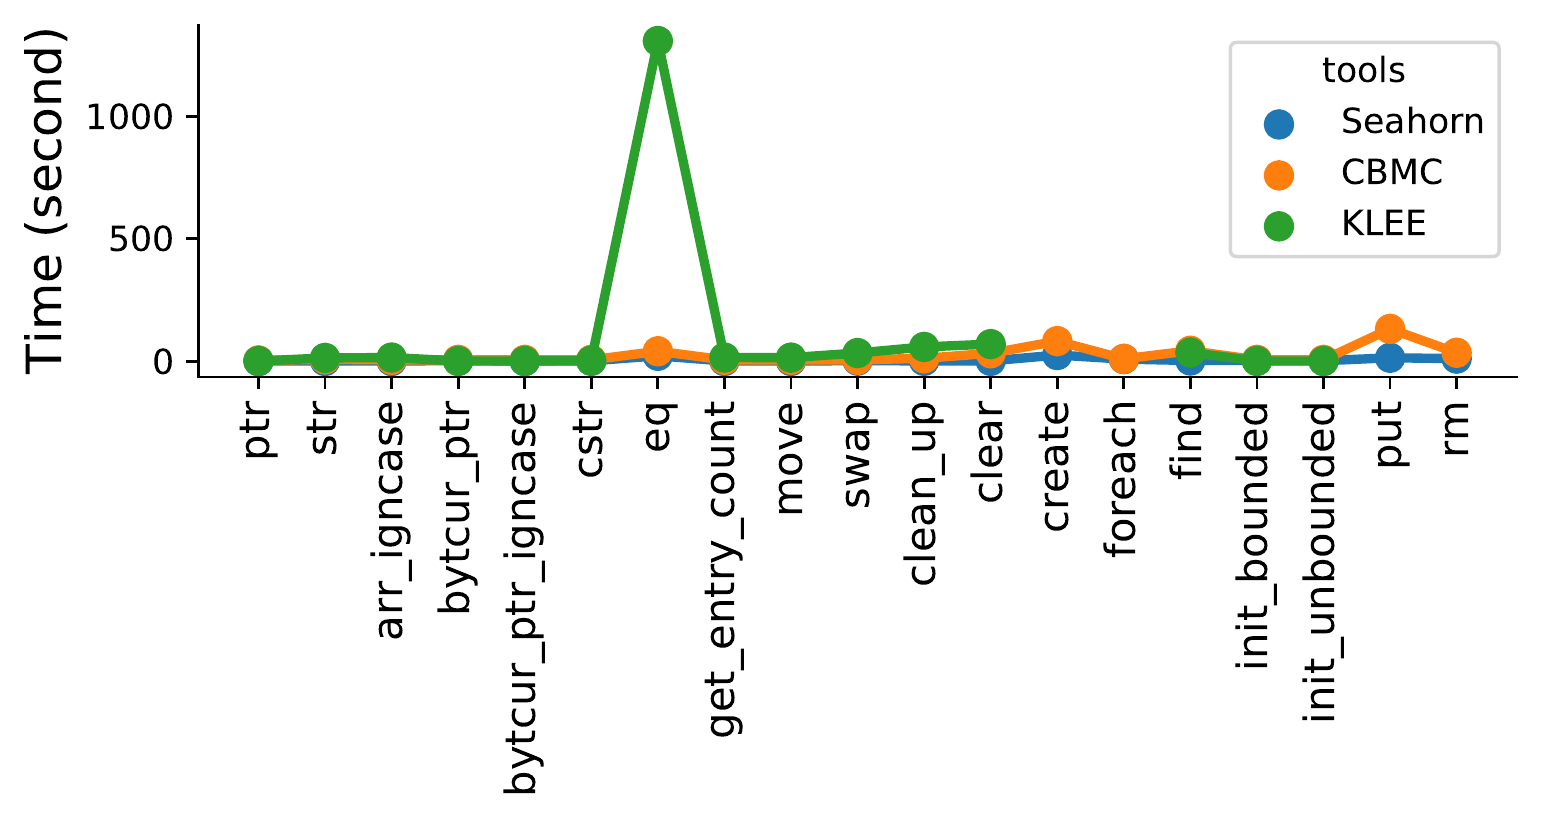}
  \caption{\code{aws_hash_table}}
  \label{fig:comp_hashtab}
\end{subfigure}%
\hfill
\begin{subfigure}{.5\linewidth}
  \includegraphics[scale=0.35]{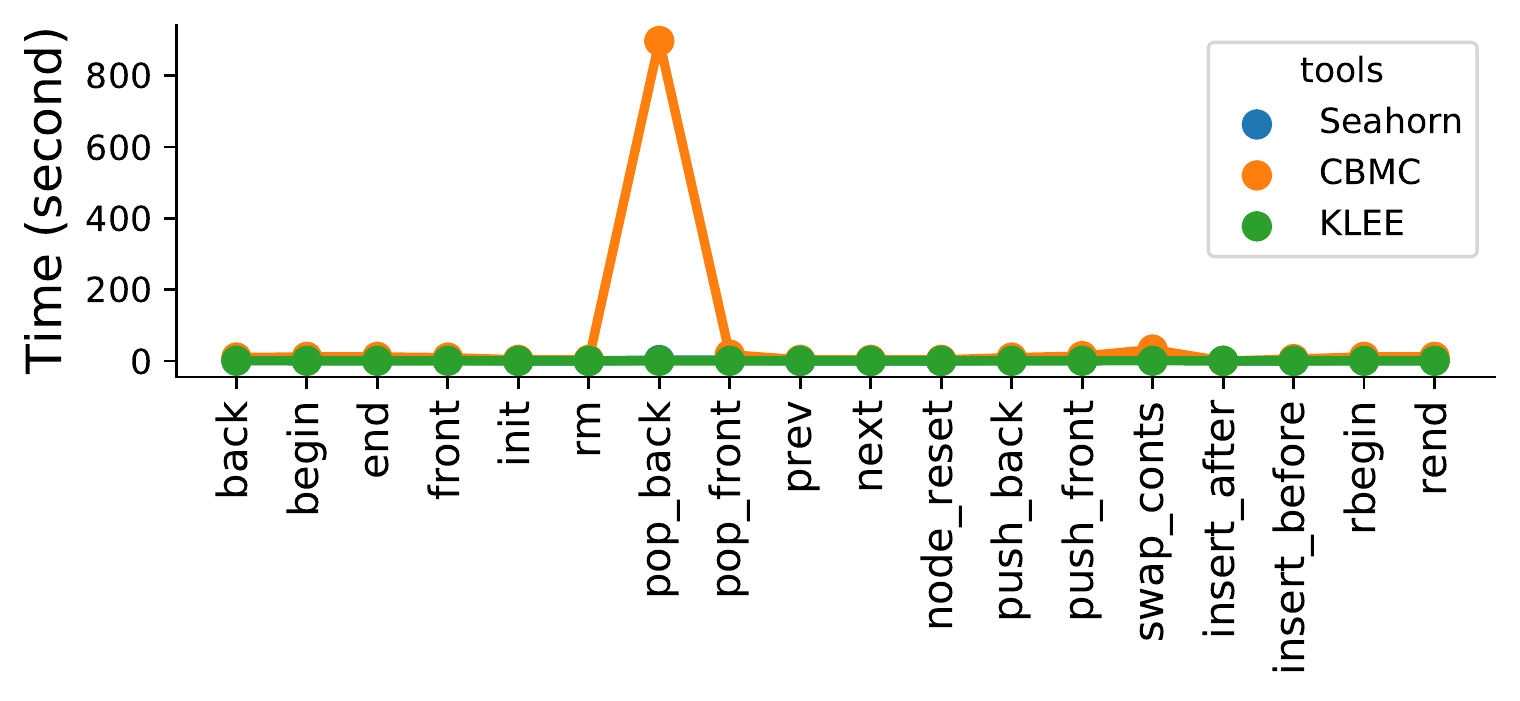}
  \caption{\code{aws_linked_list}}
  \label{fig:comp_linklst}
\end{subfigure}%
\begin{subfigure}{.5\linewidth}
  \includegraphics[scale=0.38]{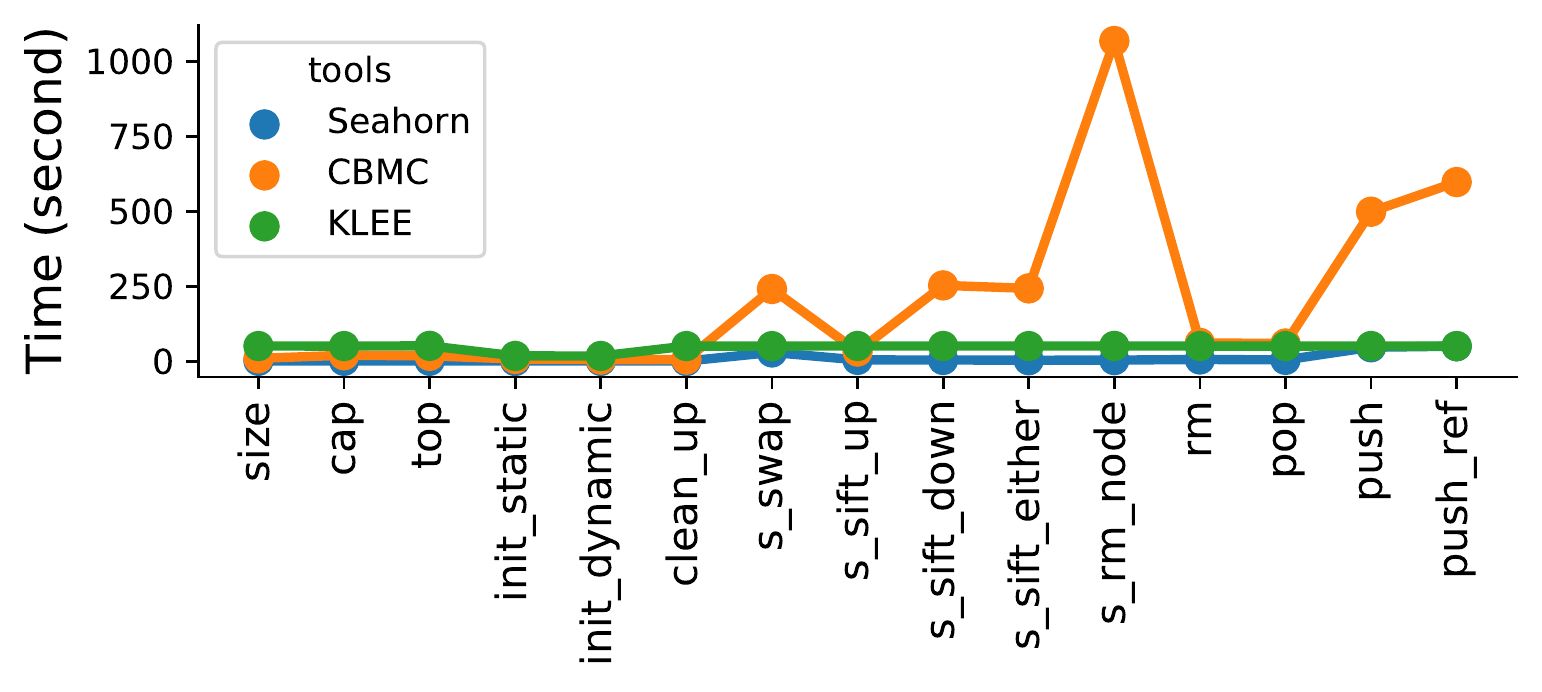}
  \caption{\code{aws_priority_queue}}
  \label{fig:comp_prioque}
\end{subfigure}%
\hfill
\begin{subfigure}{.5\linewidth}
  \includegraphics[scale=0.38]{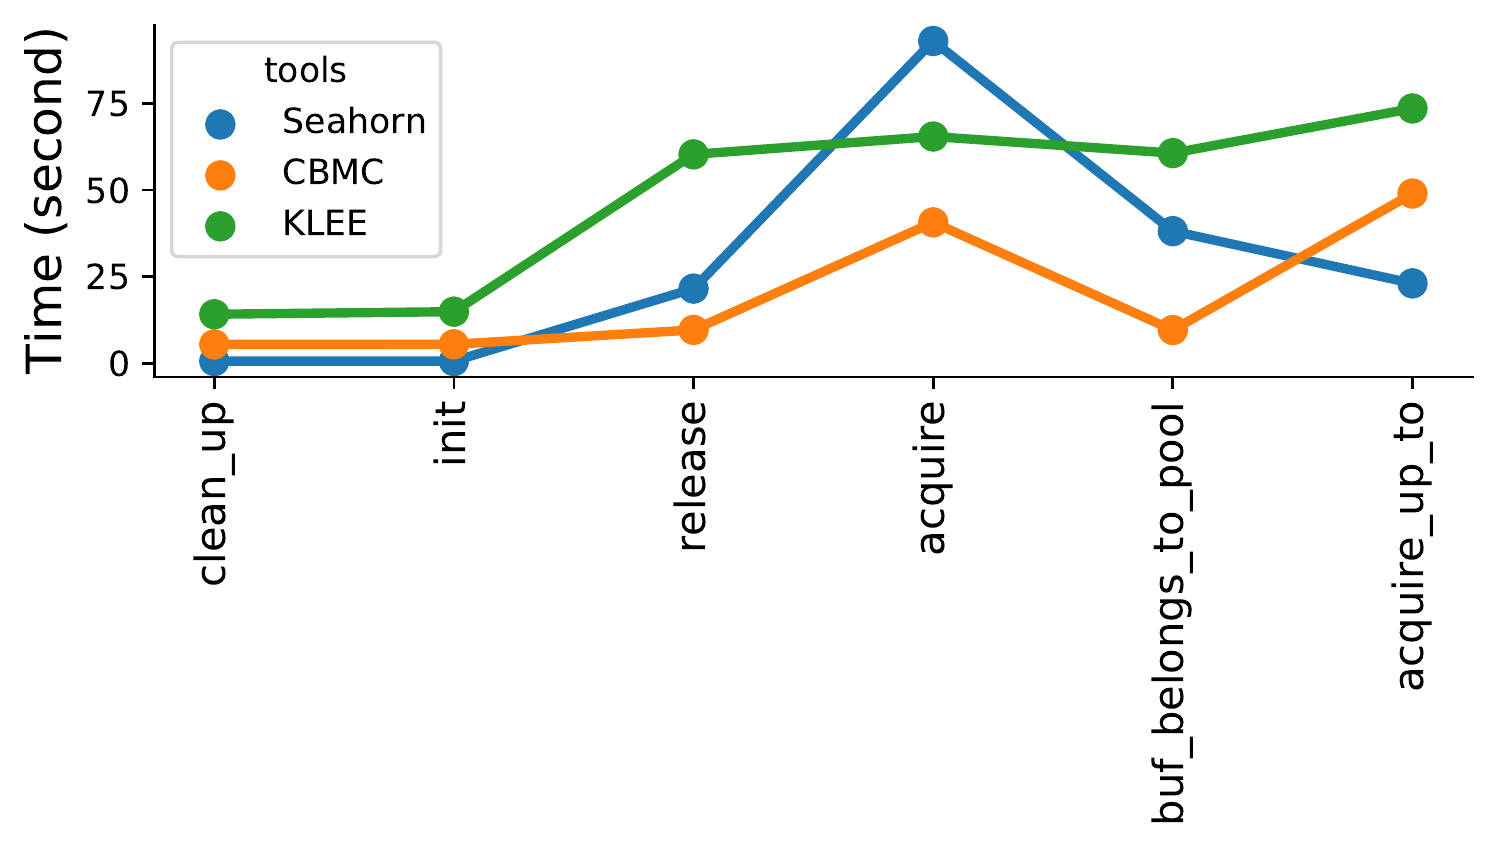}
  \caption{\code{aws_ring_buffer}}
  \label{fig:comp_ringbuf}
\end{subfigure}%
\begin{subfigure}{.5\linewidth}
  \includegraphics[scale=0.35]{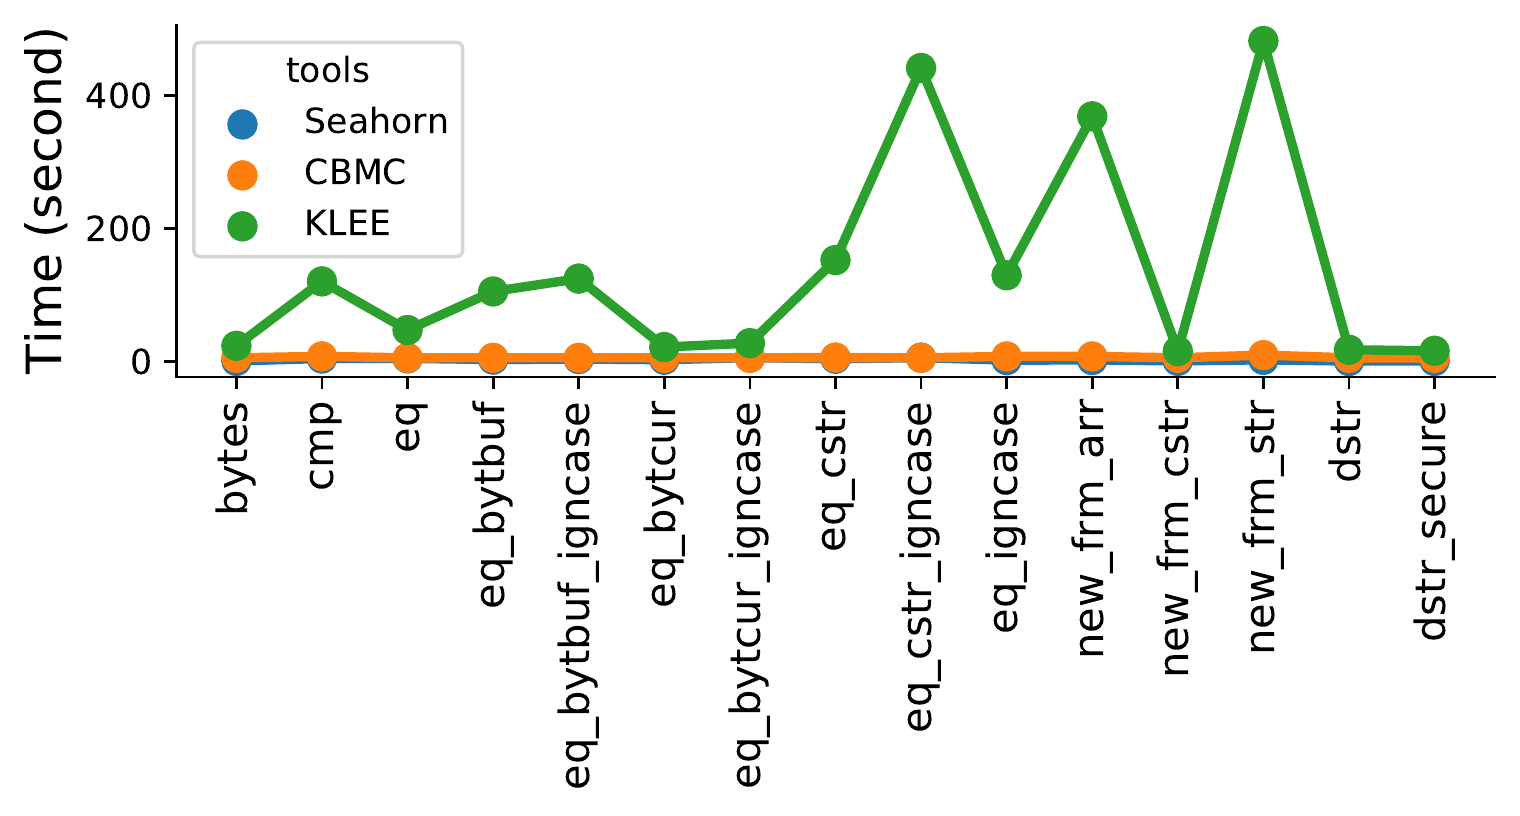}
  \caption{\code{aws_string}}
  \label{fig:comp_string}
\end{subfigure}%
\caption{Running times for \cbmc, \seahorn, and \klee on \awsccommon.}
\label{fig:comp_graphs}
\end{figure}
