# Supplementary material for: Verifying Verified Code
Source: arXiv:2107.00723 source file (2021-07-01)
Supplement: Supplementary file 11 [file setup.tex]

\subsection{Experiment and setup}
\label{sec:exper-setup}
\paragraph{Background.} In initial case study~\cite{DBLP:conf/icse/ChongCKKMSTTT20}, it does not describe detailed of performace,
We set timeout as $2000$ seconds per unit proofs

\paragraph{Verification target.} As description of ~
