# Supplementary material for: Verifying Verified Code
Source: arXiv:2107.00723 source file (2021-07-01)
Supplement: Supplementary file 13 [file fig-init-helpers.tex]

\iffalse
\newsavebox{\figseainitlstbox}
\begin{lrbox}{\figseainitlstbox}%
  \begin{lstlisting}[escapechar=@, numbers=none]
    size_t len = nd_size_t();
    size_t cap = nd_size_t();
    assume(len <= cap);
    assume(cap <= MAX_BUFFER);

    buf->len = len;
    buf->capacity = cap;
    buf->buffer = can_fail_malloc(
      cap * sizeof(*(buf->buffer)));
    buf->allocator = sea_allocator();
  
  
  
  
    @ @
  \end{lstlisting}
\end{lrbox}%

\newsavebox{\figkleeinit}
\begin{lrbox}{\figkleeinit}%
  \begin{lstlisting}
    size_t cap = nd_size_t();
    assume(cap <= MAX_BUFFER);
    buf->buffer = can_fail_malloc(
      cap * sizeof(*(buf->buffer)));
    if (buf->buffer) {
        size_t len = nd_size_t();
        assume(len <= cap);
        buf->len = len;
        buf->capacity = cap;
    }
    else {
        buf->len = 0;
        buf->capacity = 0;
    }
    buf->allocator = sea_allocator();
  \end{lstlisting}
\end{lrbox}%

\newsavebox{\figfuzzinit}
\begin{lrbox}{\figfuzzinit}%
  \begin{lstlisting}[escapechar=@,numbers=none]
      size_t len = nd_size_t();
      size_t cap = nd_size_t();
      cap %= MAX_BUFFER;
      cap = cap == 0 ? 1 : cap;
      len %= cap;
    
      buf->len = len;
      buf->capacity = cap;
      buf->buffer = can_fail_malloc(
        cap * sizeof(*(buf->buffer)));
      buf->allocator = sea_allocator();



      @ @
  \end{lstlisting}
\end{lrbox}%

\begin{figure}[t]
  \centering
  \begin{subfigure}[t]{0.3\textwidth}
  \scalebox{0.7}{\usebox{\figkleeinit}}
  \caption{for \klee} 
  \label{fig:init-klee}
  \end{subfigure}
  \hfill
  \begin{subfigure}[t]{0.3\textwidth}
  \scalebox{0.7}{\usebox{\figseainitlstbox}}
  \caption{for \seahorn} 
  \label{fig:init-sea}
  \end{subfigure}
  \hfill
  \begin{subfigure}[t]{0.3\textwidth}
  %\vspace{0.6in}
  \scalebox{0.7}{\usebox{\figfuzzinit}}
  \caption{for \libfuzzer} 
  \label{fig:init-fuzz}
  \end{subfigure}
  \caption{Tool-specific implementations for \code{initialize_byte_buf}.} 
  \label{fig:init-impls}
  \end{figure}
\fi
