# Supplementary material for: Verifying Verified Code
Source: arXiv:2107.00723 source file (2021-07-01)
Supplement: Supplementary file 14 [file initialization_helpers.tex]

\iffalse
\subsection{Adapting Initialization Functions}
\label{sec:rewrite-init-funcs}

\paragraph{Background.} In the original \cbmc case study
\cite{DBLP:conf/icse/ChongCKKMSTTT20}, due to the special semantics accepted by \cbmc, 
pre-conditions regarding data structures
 are specified in combination of the two following ways:
\begin{enumerate}
  \item primitive type fields are left uninitialized and constrained by Boolean functions 
  placed in \emph{assumptions},
  \item pointer fields are explicitly allocated in verification library functions named 
  with the pattern \code{ensure_<data-structure>_has_allocated_<field>}.
\end{enumerate}
However, as discussed in \cref{sec:questions}, this approach is inconsistent with 
\emph{de facto} C semantics and makes migrating \cbmc proofs to other tools \emph{as is} infeasible. 
In this case study, the initialization process of data structures is re-organized 
into part of \CaS. In specific, they are adapted to a set of 
verification library functions named \code{initialize_<data-structure>}. 


\paragraph{Implementations.} The new  initialization functions require different 
implementations for different tools due to differences in verification methodology. As an example, different implementations 
of \code{initialize_byte_buf} are shown in \cref{fig:init-impls}, each implementation adapting 
to \seahorn, \klee, and \libfuzzer.

\vspace{0.1in}
\bparagraph{\seahorn} initialization functions assign data structure fields with 
return values of \code{nd_<type>} functions to mark the fields as non-deterministic. 
Pre-conditions such as basic representation invariants (i.e. length should be less or 
equal to capacity) and upper bound of data structure size are specified with \emph{assumptions}.
Memory allocation functions like \code{can_fail_malloc} invokes \code{memhavoc} to 
mark content of allocated memory region as non-deterministic.

\vspace{0.1in}
\bparagraph{\klee} assumes symbolic values for program inputs instead of acquiring actual inputs for execution. To adapt initialization of non-determined variables, taking line~1 and line~6 as examples, the \code{nd_<type>} functions for \klee are implemented respectively by constructing a symbolic value which depends on given type. Moreover, in case of introducing provable false assumptions, another adaptation made gives an early exit of those program paths that contain unfitting function specifications. For example, line~12--13 apply the strictly assignment for length and capacity as zero if \code{can_fail_malloc} failed to process memory allocation. However, if the above adaptation not held, it is impossible to construct a precondition after initialization because there exists an infeasible path where \code{byte_buf} is a null reference but length and capacity are not concertized as zero. Based on this implementation, \klee allows to perform same initialization as unit proofs expected.

\vspace{0.1in}
\bparagraph{\libfuzzer} does not support non-determinism, so a different set of 
\code{nd_<type>} function implementations are created for fuzzing. The \code{nd_<type>} 
functions for fuzzing extract random data bytes generated by \libfuzzer and convert 
the bytes into correct \code{type} before returning them. \emph{Assumptions} using the 
signature \code{assume(X)} is also given a fuzzing-specific implementation, which aborts current 
fuzzing run if \code{X} evaluates to \code{false}. This behaviour is not efficient since aborting at initialization stage would result in very 
low coverage for a given input. To utilize as many generated inputs as possible, \libfuzzer 
implementations of initialization functions instead try explicitly re-assigning fields 
that with values that satisfy corresponding pre-conditions. For example, in line~3 of \cref{fig:init-fuzz}, 
\code{cap} is re-assigned to the modulo of \code{MAX_BUFFER} if \libfuzzer generated 
a value exceeding \code{MAX_BUFFER}. This way, code after line~3 will always be executed 
regardless of the return value of \code{nd_size_t()} in line~1.
\fi
