# Supplementary material for: Verifying Verified Code
Source: arXiv:2107.00723 source file (2021-07-01)
Supplement: Supplementary file 15 [file rewrite_linked_list.tex]

\iffalse
\subsection{Rewriting linked list specifications}
\label{sec:rewrit-linked-lst}
%\yb{is it possible to present this in a way that is similar to software library? e.g., a table lists the signature and description of the functions?}
\paragraph{Background.} 
% A large proportion of \awsccommon functions verified in 
% this case study are \emph{pure functions} that do not apply any side-effects 
% on the data structure they operate on. Other functions may modify certain parts 
% of a data structure, but their correctness still relies on the non-modification 
% on other parts of the same data structure. Therefore, one of the most common post 
% conditions we maintain or add when migrating CBMC proofs to use \seahorn 
% is non-modification of either all or part of the data structure under verification.
A common pattern in \emph{unit proofs} is to assume the representation invariant 
of a data structure, and to assert it after invocation of the function under 
verification along with other properties that must be maintained by the function. 
For example, the \cbmc unit proof for \code{aws_linked_list_front} shown in \cref{fig:linked_list_front_before} 
checks that the returned value is indeed the \code{next} node of \code{head}. However, 
other properties in the representation invariant can be harder to check. For example, 
checking nodes including \code{front} are \emph{unchanged} after invoking \code{aws_linked_list_front} 
on the linked list requires iterating through the linked list because the linked list 
data structure does not support constant time random access. This iterative approach is not 
ideal because loops grow program states linearly with regard to the size 
of linked lists under verification, which hinders the efficiency of unit proofs. 
Also, functions like \code{aws_linked_list_front} have \emph{O(1)} time complexity: 
per design, they only access \emph{one} 
node \emph{x}, where \emph{x} is either \code{head}, \code{tail} or a node \emph{c} levels deep 
from \code{head} or \code{tail} and \emph{c} is constant and finite. 
It does not make sense for \CaS used to verify \emph{O(1)} functions to have \emph{O(n)} time 
complexity. By observing the fact that functions similar to \code{aws_linked_list_front} only access 
finite and constant amount of memory reachable from the argument data structure, we propose 
an alternative pattern to construct and verify \code{aws_linked_list}.

\paragraph{Implementation.} To verify representation invariant of \code{aws_linked_list} 
used as argument to \emph{O(1)} \code{aws_linked_list} functions, 
we initialize a dummy \code{aws_linked_list} instances in a special manner. Starting from \code{head} node or \code{tail} node, 
only up to two nodes will be initialized as concrete \code{aws_linked_list_node} instances, 
the \code{prev} or \code{next} pointer of the last concrete node will be initialized 
as a non-deterministic pointer with the signature \code{nd_voidp()}. The reasoning for 
this design is because all \emph{O(1)} \code{aws_linked_list} functions only access 
up to two nodes reachable from \code{head} or \code{tail}. This pattern results in \emph{O(1)} \CaS 
since only constant and finite numbers of concrete nodes need to be checked in the post-condition. 
If a wrong or malicious implementation of an \emph{O(1)} \code{aws_linked_list_node} 
function attempts to access and modify any node beyond the concrete nodes, it would 
dereference a non-deterministic node and cause a memory 
safety failure detectable by \seahorn, causing the verification task to return a negative result.

To make this pattern more accessible to verification engineers and developers, we created three sets 
of helper API functions, each set of functions 
adapts to a different way \emph{constant time linked list access} functions access linked lists:
access from the head only, access from the tail only or access from both the head and the tail. The APIs come with 
suggestive names:
\code{sea_nd_init_aws_linked_list_*} functions construct dummy \code{aws_linked_list} 
instances with non-deterministic length. \cref{fig:dll} illustrates how a dummy \code{aws_linked_list} with length greater 
than two would be constructed under each access scenario. \code{aws_linked_list_save_*} functions 
save concrete linked list nodes from a dummy \code{aws_linked_list}. \code{is_aws_list_unchanged_*} functions 
are then used in the post-condition to check concrete nodes are not modified. \cref{fig:linked_list_front_after} 
shows the rewritten unit proof for \code{aws_linked_list_front}. Note that not only is 
the rewritten version more efficient than the original \cbmc proof, but it also contains 
\emph{stronger} specifications. For example, if \code{aws_linked_list_front} tries to 
remove or modify a node in the linked list, the rewritten proof would catch this behaviour, while 
the original proof only checks whether the returned value is correct and whether 
the linked list is well formed.



\newsavebox{\figlistbox}
\begin{lrbox}{\figlistbox}%
  \begin{lstlisting}
    void aws_linked_list_front_harness() {
    /* data structure */
    struct aws_linked_list list;

    ensure_linked_list_is_allocated(&list, MAX_LINKED_LIST_ITEM_ALLOCATION);

    /* Keep the old last node of the linked list */
    struct aws_linked_list_node *old_first = list.head.next;

    /* Assume the preconditions. The function requires that list != NULL */
    __CPROVER_assume(!aws_linked_list_empty(&list));

    /* perform operation under verification */
    struct aws_linked_list_node *front = aws_linked_list_front(&list);

    /* assertions */
    assert(aws_linked_list_is_valid(&list));
    assert(aws_linked_list_node_prev_is_valid(front));
    assert(aws_linked_list_node_next_is_valid(front));
    assert(front == old_first);
}
  \end{lstlisting}
\end{lrbox}%

\begin{figure}[t]
  \centering
  \scalebox{0.8}{\usebox{\figlistbox}}
  \caption{\cbmc unit proof for \code{aws_linked_list_front}.} 
  \label{fig:linked_list_front_before}
\end{figure}


\begin{figure}[t]
  \centering
  \includegraphics[scale=0.8]{graph/linked_list_dummy.pdf}
  \caption{Dummy linked lists for proofs.}
  \label{fig:dll}
\end{figure}

\fi
\iffalse
\newsavebox{\figlistmainbox}
\begin{lrbox}{\figlistmainbox}%
  \begin{lstlisting}
    int main() {
      /* data structure */
      struct aws_linked_list list;
      struct saved_aws_linked_list to_save = {0};
      size_t size;

      sea_nd_init_aws_linked_list_from_head(&list, &size);
      struct aws_linked_list_node *start = &list.head;
      aws_linked_list_save_to_tail(&list, size, start, &to_save);

      // precondition in function does not accept empty linked list
      assume(!aws_linked_list_empty(&list));

      /* perform operation under verification */
      struct aws_linked_list_node *front = aws_linked_list_front(&list);

      /* assertions */
      sassert(list.head.next == front);
      sassert(aws_linked_list_node_prev_is_valid(front));
      sassert(aws_linked_list_node_next_is_valid(front));
      sassert(is_aws_list_unchanged_to_tail(&list, &to_save));

      return 0;
    }
  \end{lstlisting}
\end{lrbox}%


\begin{figure}
  \centering
  \scalebox{0.8}{\usebox{\figlistmainbox}}
  \caption{\seahorn unit proof for \code{aws_linked_list_front}.} 
  \label{fig:linked_list_front_after}
\end{figure}
\fi

%%% Local Variables:
%%% mode: latex
%%% TeX-master: "paper"
%%% End:
