# Supplementary material for: Verifying Verified Code
Source: arXiv:2107.00723 source file (2021-07-01)
Supplement: Supplementary file 16 [file spec_rewrites.tex]

\iffalse
\section{Description of major specification rewrites}
\label{sec:spec_rewrites}
\input{appendix/spec_rewrite/rewrite_linked_list}
\input{appendix/spec_rewrite/fig-init-helpers}
\input{appendix/spec_rewrite/initialization_helpers}
\fi
